# Supplementary material for: Signed Graph Metric Learning via Gershgorin Disc Perfect Alignment
Source: arXiv:2006.08816 source file (2021-06-11)
Supplement: Supplementary file 1 [file appendix.tex]

\newpage

\section{Gershgorin Disc Alignment}

\begin{figure}
\begin{center}
\includegraphics[width=1.8in]{fig/pseudo-bipartite.png}
\vspace{-0.1in}
\caption{Example of a 5-node balanced graph.}
\label{fig:pseudo-bipartite}
\end{center}
\end{figure}

Consider an irreducible and balanced signed graph $\cG(\cN,\cE^+ \cup \cE^-,\cU)$ with nodes $\cN$, positive and negative inter-node edges, $\cE^+$ and $\cE^-$, and self-loops $\cU$. 
A balanced graph $\cG$ means that $\cG$ has no cycle of odd number of negative edges, and
according to the Cartwright-Harary Theorem \red{add ref}, nodes $\cN$ can be colored into red and blue, so that a negative edge always connects a red node and a blue node. 
As an example, consider the 5-node balanced graph in Fig.\;\ref{fig:pseudo-bipartite}, where nodes 1, 2 and 5 are colored blue, while nodes 3 and 4 are colored red.
Notice that only positive edges connect nodes of the same colors, while negative edges connect nodes of the opposite colors. 

Denote the sets of red and blue nodes in $\cG$ by $\cN_r$ and $\cN_b$ respectively, where $\cN_r \cap \cN_b = \emptyset$ and $\cN_r \cup \cN_b = \cN$.  
Each inter-node edge $(i,j) \in \cE^+ \cup \cE^-$ has weight $w_{i,j} \in \mathbb{R}, i \neq j$. Each node $i$ has a self-loop with weight $u_i = w_{i,i} \in \mathbb{R}$ (possibly 0). 
%that satisfies 
%\begin{align}
%u_{i} &> - \sum_{j \,|\, (i,j) \in \cE^+ \cup \cE^-} w_{i,j}
%\label{eq:append0}
%\end{align}

The \textit{adjacency} matrix $\W$ contains the inter-node edge weights $w_{i,j}$ in the off-diagonals and the self-loop weights $u_i$ on the diagonals.
The \textit{degree} matrix $\D$ is a diagonal matrix where $d_{i,i} = \sum_{j} w_{i,j}$. 
Denote by $\M$ the \textit{generalized graph Laplacian} matrix of graph $\cG$ computed as 
\begin{align}
\M = \D - \W + \text{diag}(\W)
\end{align}

Denote by $\B$ a similar transform of $\M$ via diagonal matrix $\S = \text{diag}(s_1, \ldots, s_N)$, where $s_i \neq 0, \forall i$, \ie, 
\begin{align}
\B = \S \M \S^{-1}
\end{align}
Denote by $\v$ the first eigenvector of $\M$ corresponding to graph $\cG$---\ie, $\M \v = \lambda_{\min} \v$, where $\lambda_{\min}$ is the smallest eigenvalue of $\M$.
We make the following claim as a theorem:
\begin{theorem}
If $s_i = 1/v_i$, where $v_i \neq 0, \forall i$, then left-ends of $\B$'s Gershgorin discs are aligned at $\lambda_{\min}$. 
\end{theorem}
We prove this claim as follows.

\vspace{0.1in}
We define a positive-edge-only graph $\cG'(\cN,\cE',\cU')$ related to signed graph $\cG$ containing the same nodes $\cN$.
$\cG'$ keeps all positive edges $\cE^+$, 
but for each negative edge $\cE^-$, $\cG'$ switches its sign to positive.
Thus,
\begin{align}
w'_{i,j} = \left\{ \begin{array}{ll}
w_{i,j} & \mbox{if}~ (i,j) \in \cE^+ \\
-w_{i,j} & \mbox{if}~ (i,j) \in \cE^- 
\end{array} \right.
\end{align}

Each node $i$ in $\cG'$ has a self-loop with (possibly 0) weight $u'_{i}$ defined as
\begin{align}
u'_{i} &= u_{i} + 2 \sum_{j \,|\, (i,j) \in \cE^-} w_{i,j}
\end{align}
Thus, a red / blue node $i \in \cN$ that has no connection to nodes of opposite colour has the same self-loop $u'_{i} = u_{i}$ as $\cG$.

For each graph signal $\y$ on $\cG'$, we define a corresponding signal $\x$ on $\cG$, where
\begin{align}
x_i = \left\{ \begin{array}{ll}
-y_i & \mbox{if}~ i \in \cN_r \\
y_i & \mbox{if}~ i \in \cN_b
\end{array} \right.
\label{eq:append1}
\end{align}
We first show that $\x^{\top} \M \x = \y^{\top} \M' \y$.
The quadratic form $\y^{\top} \M' \y$ can be written as
\begin{align}
=& \sum_{(i,j) \in \cE^+ \cup \cE^-} w'_{i,j} (y_i - y_j)^2 + \sum_{i \in \cN} u'_{i} y_i^2 \nonumber \\
\stackrel{(a)}{=}& \sum_{(i,j) \in \cE^+} w'_{i,j} (y_i - y_j)^2 
+ \sum_{(i,j) \in \cE^-} w'_{i,j} 
\left( y_i^2 + y_j^2 \right)
\nonumber \\
& - \sum_{(i,j) \in \cE^-} w'_{i,j} 
2 y_i y_j + 
\sum_{i \in \cN} u'_{i} y_i^2 \nonumber \\
\stackrel{(b)}{=}& \sum_{(i,j) \in \cE^+} w_{i,j} (x_i - x_j)^2
- \sum_{(i,j) \in \cE^-} w_{i,j} 
\left( x_i^2 + x_j^2 \right) \nonumber \\
& - \sum_{(i,j) \in \cE^-} w_{i,j} 
2 x_i x_j + \sum_{i \in \cN} \left( u_{i}
+ 2 \sum_{j | (i,j) \in \cE^-} w_{i,j} \right) x_i^2
\nonumber \\
\stackrel{(c)}{=}& \sum_{(i,j) \in \cE^+} w_{i,j} (x_i - x_j)^2
- \sum_{(i,j) \in \cE^-} w_{i,j} 
\left( x_i^2 + x_j^2 \right) \nonumber \\
& - \sum_{(i,j) \in \cE^-} w_{i,j} 
2 x_i x_j + \sum_{i \in \cN} u_{i} x_i^2
+ 2 \!\! \sum_{(i,j) \in \cE^-} w_{i,j} (x_i^2 + x_j^2)
\nonumber \\
\stackrel{(d)}{=}& \!\!
\sum_{(i,j) \in \cE^+} w_{i,j} (x_i - x_j)^2 + \!\!\!\!
\sum_{(i,j) \in \cE^-} w_{i,j} (x_i - x_j)^2 + \sum_{i\in\cN} u_i x_i^2 
\nonumber \\
=& \x^{\top} \M \x
\end{align}
In $(a)$, we write the sums for positive and negative edges separately, and expand the quadratic term $(y_i - y_j)^2$ for negative edges.
In $(b)$, the first term follows since edge $(i,j) \in \cE^+$ connects two nodes of the same colour, and the third term follows since only one of $i$ and $j$ is a red node. 
In $(c)$, the last term is a rewriting of $\sum_{i \in \cN} \sum_{j|(i,j)\in\cE^-} w_{i,j} x_i^2$.
In $(d)$, the second term combines the second, third and fifth terms in $(c)$. 

The corollary of $\x^{\top} \M \x = \y^{\top} \M' \y$ is that given the first eigenvector $\y^*$ that minimizes the Rayleigh quotient of $\M'$:
\begin{align}
\y^* = \min_{\y} \frac{\y^{\top} \M' \y}{\y^{\top} \y},
\end{align}
the corresponding $\x^*$ in (\ref{eq:append1}) also minimizes the Rayleigh quotient of $\M$, and thus is the first eigenvector of $\M$.

Finally, we define a shifted graph Laplacian matrix $\cL = \M' + \epsilon \I$, where constant $\epsilon > 0$ is
\begin{align}
\epsilon &> \max_{i} \left\{ 
- \sum_{j \,|\, (i,j) \in \cE^+ \cup \cE^-} w_{i,j} - u_i
\right\}
\label{eq:append0}
\end{align}
$\cL$ has the same set of eigenvectors as $\M'$, and its eigenvalues are the same as $\M'$ but shifted up by $\epsilon$. 

We see that $\cL$ has strictly positive node degrees $\delta_i$, \ie, 
\begin{align}
\delta_i &= \sum_{j | (i,j) \in \cE'} w'_{i,j} + u'_{i} + \epsilon \nonumber \\
&= \sum_{j | (i,j) \in \cE^+} w_{i,j} -
\sum_{j |(i,j) \in \cE^-} w_{i,j} +
u_i + 2 \sum_{j | (i,j) \in \cE^-} w_{i,j} + \epsilon \nonumber \\
&= \sum_{j|(i,j) \in \cE^+} w_{i,j} +
\sum_{j | (i,j) \in \cE^-} w_{i,j} + u_i + \epsilon \stackrel{(a)}{>} 0 \nonumber
\end{align}
In $(a)$, the inequality is due to the assumed inequality for $\epsilon$ in (\ref{eq:append0}).

From our previous work \cite{yang20}, we know that given $\cL$ is a generalized graph Laplacian matrix for an irreducible graph with positive edges and degrees, $\cL$'s first eigenvector (also $\M'$'s first eigenvector) $\y^*$ is a strictly positive vector, stemming from the Perron-Frobenius Theorem. 
Thus, corresponding $\x^*$ is strictly non-zero first eigenvector, \ie, $x^*_i \neq 0, \forall i$. 

Having established first eigenvector $\x^*$ of $\M$, we can define diagonal matrix $\S = \text{diag}(1/x_1, \ldots, 1/x_N)$, and write
\begin{align}
\S \M \S^{-1} \S \x^* &= \lambda_{\min} \S \x^* \\
\B \1 &= \lambda_{\min} \1
\label{eq:append2}
\end{align}
where $\B = \S \M \S^{-1}$.
Each row $i$ in (\ref{eq:append2}) states that 
\begin{align}
b_{i,i} + \sum_{j \neq i} b_{i,j} &= \lambda_{\min} \\
m_{i,i} + s_i \sum_{j \neq i} m_{i,j} / s_j &= \lambda_{\min}
\end{align}
Suppose $i$ is a red node. 
Then $x^*_i = -y^*_i < 0$, and thus $s_i = 1/x^*_i < 0$.
For each red neighbor $j$ of $i$, $s_j < 0$, and $w_{i,j} > 0$ means that $m_{i,j} < 0$.
We can hence conclude that $s_i m_{i,j} / s_j < 0$ and $s_i m_{i,j} / s_j  = - |s_i m_{i,j} / s_j|$.
For each blue neighbor $j$ of $i$, $s_j > 0$, and $w_{i,j} < 0$ means that $m_{i,j} > 0$. 
We can hence conclude also that $s_i m_{i,j} / s_j < 0$ and $s_i m_{i,j} / s_j  = - |s_i m_{i,j} / s_j|$.
Similar analysis can be performed if $i$ is a blue node.
Thus (\ref{eq:append1}) can be rewritten as 
\begin{align}
m_{i,i} - \sum_{j \neq i} | s_i m_{i,j} / s_j| = \lambda_{\min}
\end{align}
In other words, left-end of $\B$'s $i$-th Gershgorin disc---centre $m_{i,i}$ minus radius $\sum_{j \neq i} | s_i m_{i,j} / s_j|$---is aligned at $\lambda_{\min}$.
This holds true for all $i$. $\square$
